# Supplementary material for: Binocular Model: A deep learning solution for online melt pool temperature analysis using dual-wavelength Imaging Pyrometry
Source: arXiv:2408.11126 source file (2024-08-26)
Supplement: Supplementary file 1 [file 10_appendix.tex]

\appendix

% %%
% %% The next two lines define the bibliography style to be used, and
% %% the bibliography file.
% \bibliographystyle{Reference-Format}
% \bibliography{references}
% %%
% %% If your work has an appendix, this is the place to put it.
